# Supplementary material for: Grain Boundaries in Chemical Vapor Deposited Atomically Thin Hexagonal Boron Nitride
Source: arXiv:1811.07618 source file (2018-11-19)
Supplement: Supplementary file 1 [file Supplemental_Material.pdf]

# Supplemental Material

## Grain Boundaries in Chemical Vapor Deposited Atomically Thin Hexagonal Boron Nitride

*Xibiao Ren[1], Jichen Dong[2], Peng Yang[3], Jidong Li[4], Guangyuan Lu[3], Tianru Wu[3], Haomin Wang[3], Wanlin Guo[4], Ze Zhang[1], Feng Ding[2,5,*], Chuanhong Jin[1,†]*

[1]State Key Laboratory of Silicon Materials, School of Materials Science and Engineering Zhejiang University, Hangzhou, Zhejiang 310027 , P. R. China

[2]Centre for Multidimensional Carbon Materials, Institute for Basic Science, Ulsan 44919, Republic of Korea

[3]State Key Laboratory of Functional Materials for Informatics, Shanghai Institute of Microsystem and Information Technology, Chinese Academy of Sciences, 865 Changning Road, Shanghai 200050, P.R. China

[4]State Key Laboratory of Mechanics and Control of Mechanical Structures, the Key Laboratory of Intelligent Nano Materials and Devices of DoE, Institute of Nano Science of Nanjing University of Aeronautics and Astronautics, Nanjing 210016, China

[5]School of Materials Science and Engineering, Ulsan National Institute of Science and Technology (UNIST), Ulsan 44919, Republic of Korea

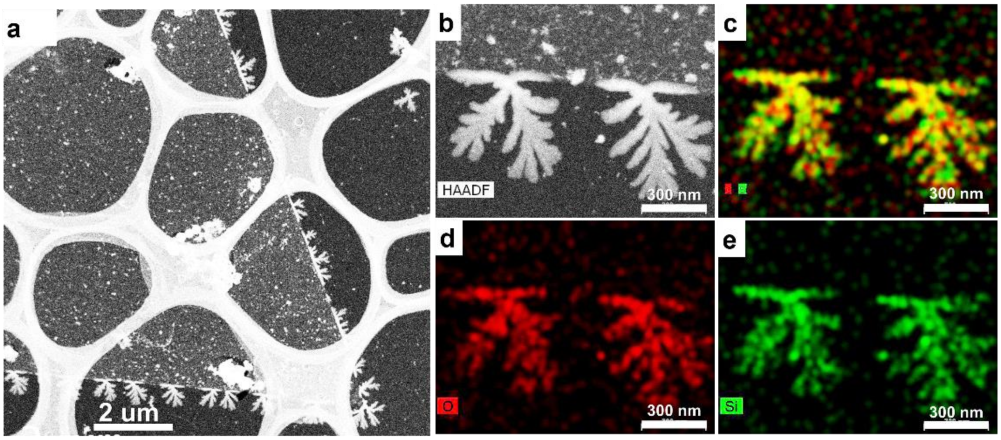


**Figure S1** (a,b) ADF-STEM images of tree-like structures at the edge of h-BN grain. (c-e) EDS mapping images which combined with e (oxygen) and f (silicon). The silicon oxide may come from the quartz tube.

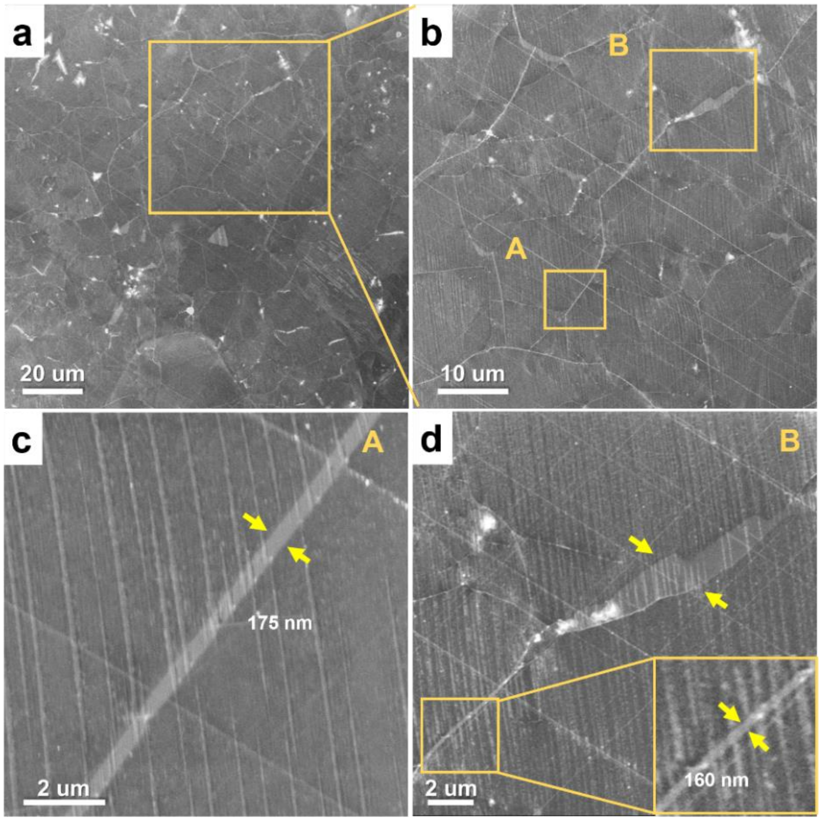


**Figure S2** (a) SEM images of continuous sample. (b-d) shown the overlapping grain boundaries.

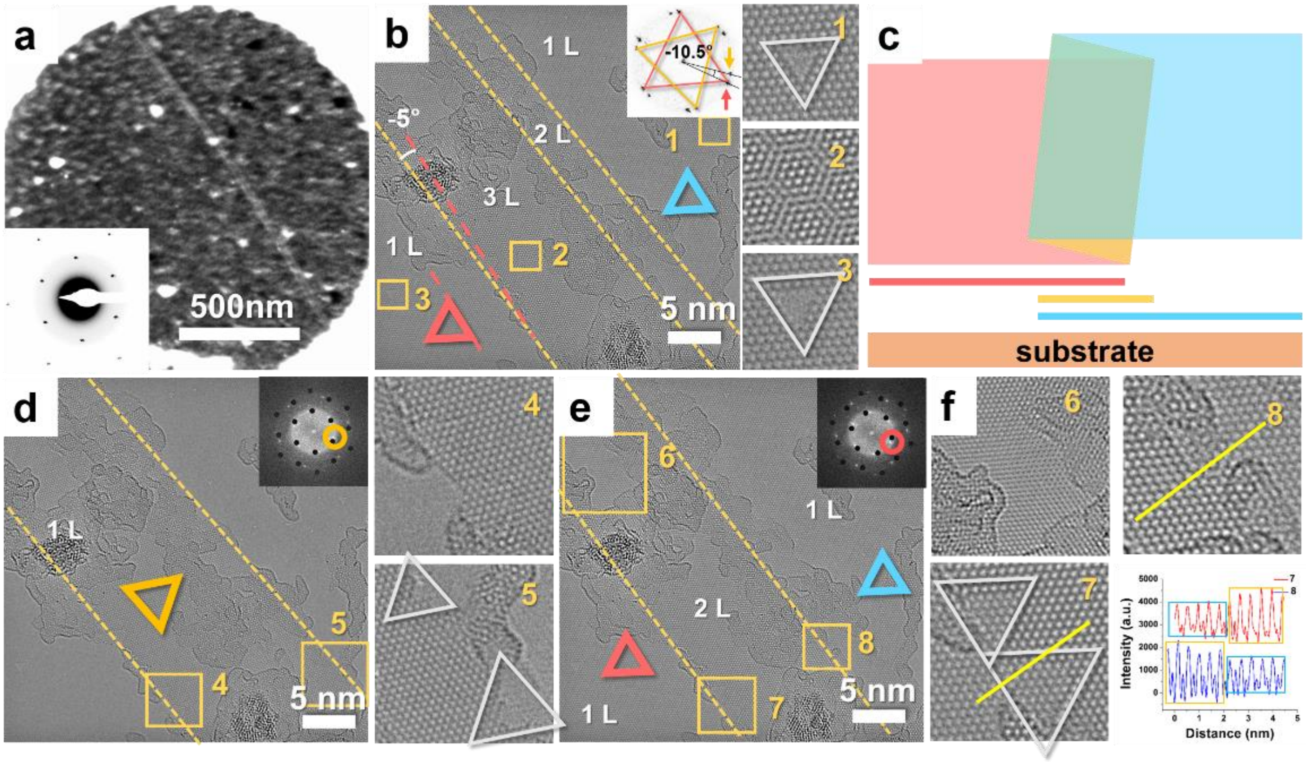


**Figure S3** (a) Dark filed image of h-BN film on holy carbon and its corresponding FFT. (b) The HRTEM image of grain boundaries in a and its local structure are displayed on the right. (c) schematic diagram of grain boundary structure in b. (d) the inverse FFT image of b, which cut the information of two top and bottom layer in c, and its local structures in certain regions are displayed on the right. The white triangle is the shape of the hole which indicates the orientations of the interlayer. (e) the inverse FFT image of b which cut the lattice information of the interlayer. (f) the local structure in e and the intensity profile which tell us the layer number of the certain areas.

To further determine the structure of 0 °-GB, we acquired images in a discrete sample on holy carbon (Figure S3), which could see the detailed atomic structure of interlayer. Note that we can not distinguish whether it was a GB between two grains or a wrinkle inside the grain because it' hard to keep the crystal

shape after sample transfer. The orientation of each layer is determined by the electron beam induced triangular holes with nitrogen terminated zigzag edges. The interlayer shows nearly opposite direction with respect to the grains. The angle between the interlayer and left grain is -10.5 °, which is two times as the angle between the GB and the boron zigzag direction. This feature confirms the structure of the GB structure of h-BN on ultrathin carbon films.

Data from discrete films on ultrathin carbon film (GB between two grains) and holy-carbon (GB or wrinkles) and continiuous films (GB or wrinkles) on holy-carbon shows similar width distribution and angle relationship as shown in Figure S4. Thus, we confirm the folded nature of 0 °-GBs.

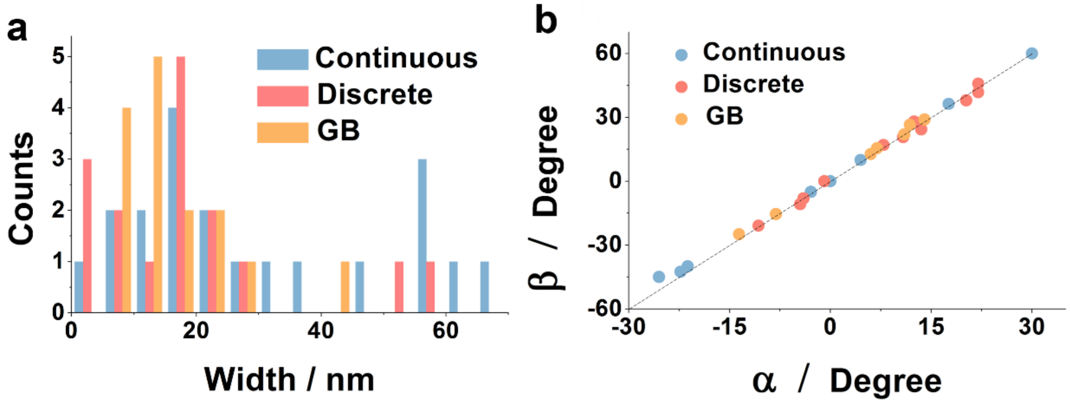


**Figure S4** (a) GBs width distributions of 0 °-GBs. The red and blue data are from the discrete and continuous films on holy carbon, which could be GBs or wrinkles. And the orange one is from the GBs in discrete films on ultrathin carbon film (b) Statistic plot of α and β values in GBs or wrinkles.

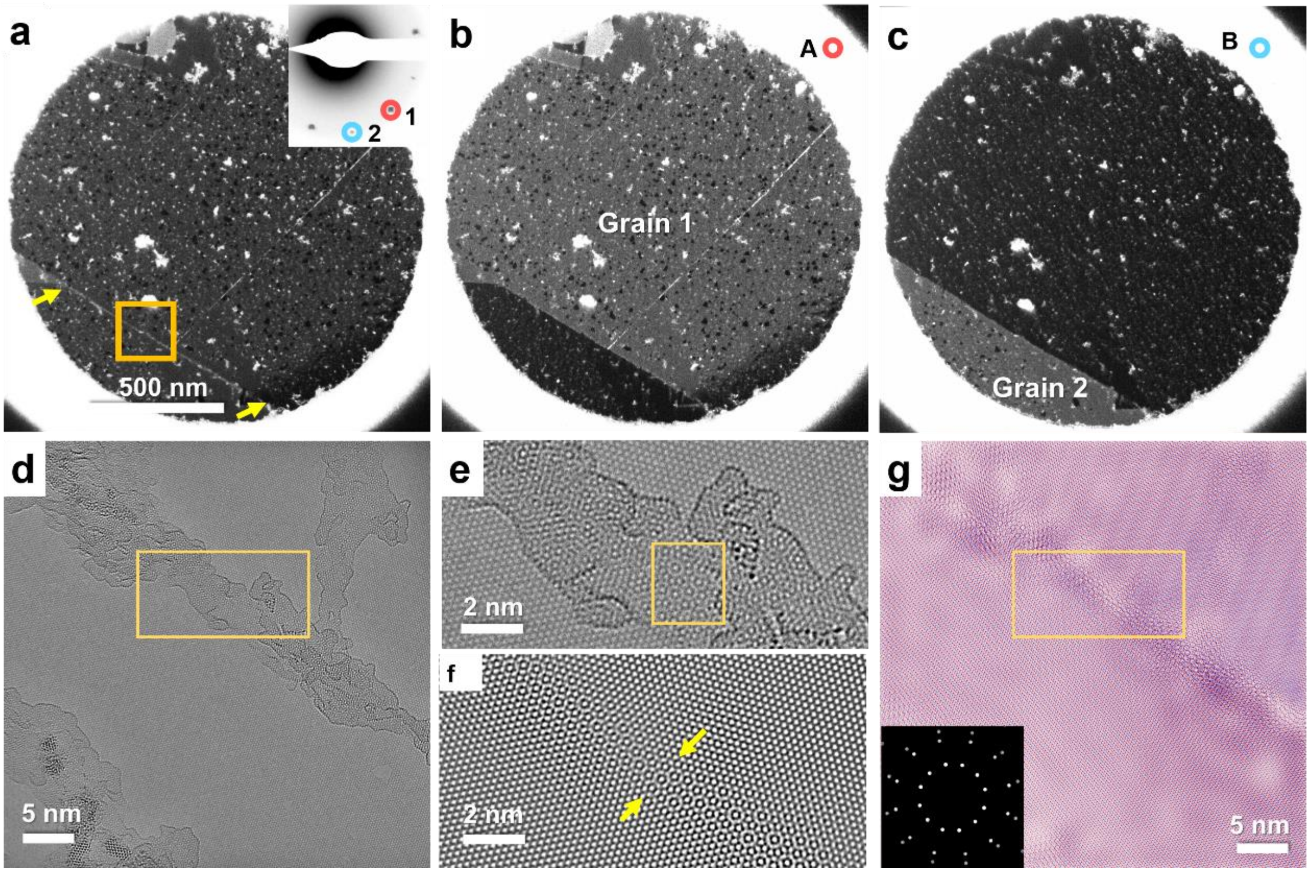


**Figure S5** (a) Dark field image which overlay of two b and c, which shows a ultranarrow GB.(d) HRTEM image in a and the its inverse FFT image in (g) which remove the contamination informations (e,f) zoom in image of the same region in d and g, it's clear that there are moire pattern in e as indicated in orange rectangle, which shows a narrow overlapped region. Note that it can not give the information of width of grain boundary from f, due to the imaging process.

It can be seen that the structure of GB formed by two grains with boron zigzag edges is different from the structure of GB formed by two grains with nitrogen zigzag edges as in Figure S6. There is a folded region which shows the similar behavior as in 0 °-GBs(-the angle of 38.5 ° is around two times as -19.5 °), while with two inverse grains on two sides as indicated in Figure S16d. Such GB structure may

be induced by the formation process as indicated in Figure 4 in the main text. The folded region may induce by the cooling process as discussed in the main text, while the structure right after the growth remains unclear.

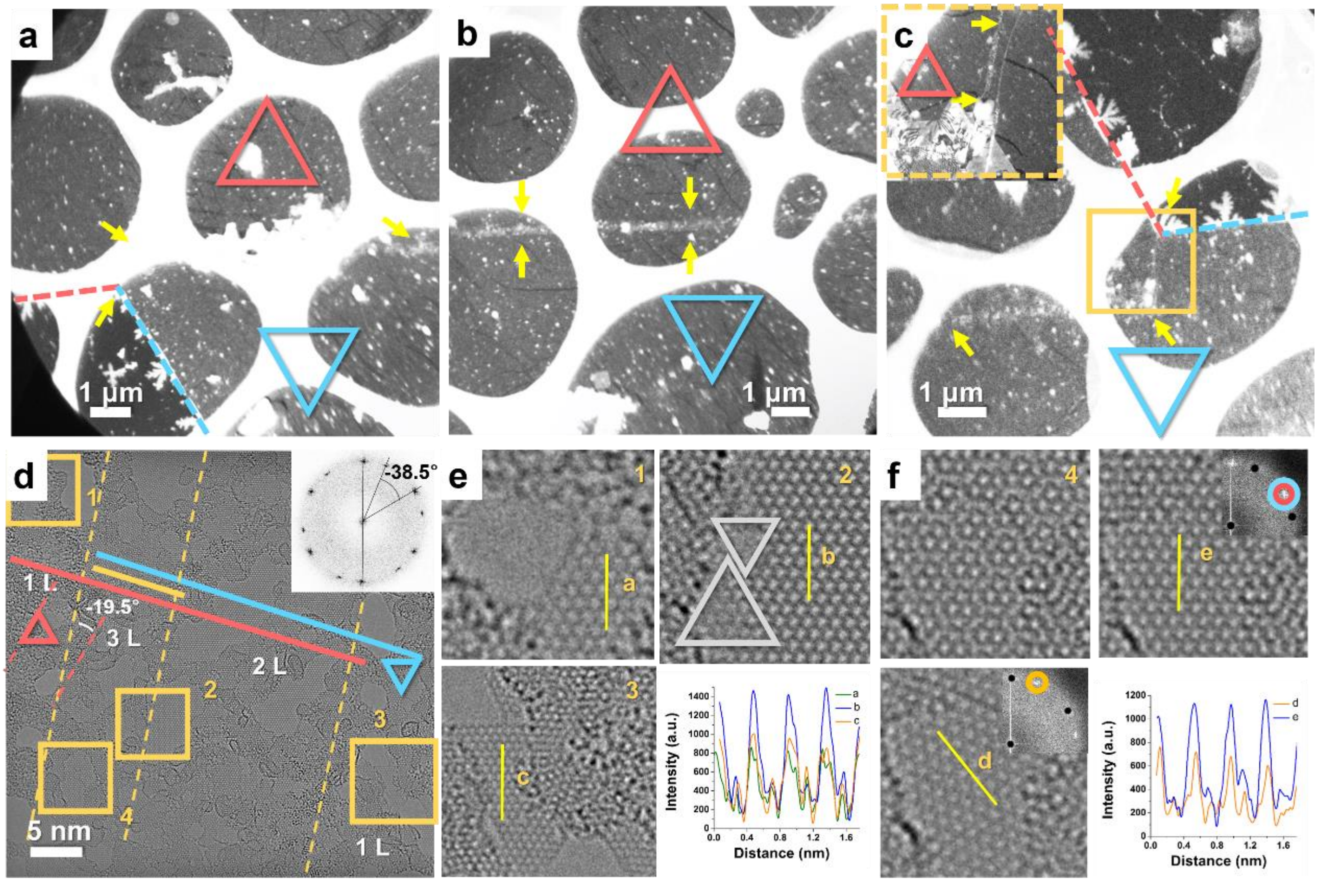


**Figure S6** (a,b,c) dark field images of 60 °-GBs at different regions. (d) HRTEM image of the region marked by the orange rectangle in c, and its corresponding FFT. (e,f) detailed structure in d as marked by numbers, the image marked by red and blue circles are the inverse FFT image of the top left image in f by the mask inserted which indicate the overlap of two grains as marked red and blue in d, while the image marked by orange circle is from the interlayer.
